# Supplementary material for: GUTS: Generalized Uncertainty-Aware Thompson Sampling for Multi-Agent Active Search
Source: arXiv:2304.02075 source file (2025-01-09)
Supplement: Supplementary file 1 [file appendix.tex]

\section{Appendix}

\subsection{Detector False Positives}
In runs 1-5, the ML detector was tuned such that it had a high precision. In runs 6 and 7, the false positive rate was set such that the GNATS was receiving several detections a minute. In both runs, GNATS proved able to reason through the incorrect information and locate all OOIs despite the sparsity requirement baked into the algorithm. This is because the act of maximising reward to choose sensing actions allows it to operate well even when OOIs are densely distributed.

\subsection{Communication Breakdown}
% Despite runs 6 and 7 being subjected to communication breakdown they emerged as the best performers in Fig. \ref{fig:result_graph}.

In run 6, we ran two UGVs with successful communication of robot locations between them but communication breakdown for OOI detections. Therefore, positive detections made by one UGV was unknown to the other. Hence, both UGVs assumed the other one only made negative observations for the entire run, which is erroneous. We felt this was a stronger test of communication breakdown as it not only encapsulated incomplete information but incorrect information too. An algorithm less resistant to noise would have skipped over regions that were assumed to have been covered by another robot but our approach was robust to it.

The number of data collection decisions per OOI found was 1. Which is the best run on this metric. The time taken is marked as an average time between the two UGVs. The last remaining OOI that remained unrecovered was on top of a hill and hence invisible to the UGVs. Hence run 6 had full recovery of OOIs.

\subsection{Hardware Failure}
In run 7 we launched two UGVs running GNATS and one UAV running random coverage. The same method of communication breakdown as run 6 was instituted. In addition to that, the detector on the UAV was disabled. The UAV's only purpose in the field was to cause the UGVs to erroneously assume negative observations for it. This test demonstrates the ability of the system to perform under hardware failure and recover all OOIs (recall that the last remaining OOI was unrecoverable for the UGVs). 

In the run 7 entry in Table \ref{table_example} we have not included time taken and data collection decision count from the UAV since it was not running GNATS nor could it contribute to the OOI count. We notice that the number of data collection decisions per OOI found deteriorated as compared to run 6. We believe this is because the search region is not large enough for three agents without major overlaps in areas covered leading to inefficiencies. A secondary reason is the greater degree of wrong information that the two working UGVs had to reason through. We did not perform a run with two UAVs and two UGVs as we expected a further degradation in performance due to the limited search space available.

In one of the runs not presented in Table \ref{table_example} (as there were no OOIs set up), a team of two UGVs were given the same search space and, close to the beginning of the run, one of the UGVs experienced a systems failure causing it to stall for the entire run. The second UGV covered the entire search space alone. This shows that without explicitly segmenting the search space GNATS is robust to total robot failures without operator intervention.

% We conducted run 5 with a single UAV running the full GNATS algorithm which led to another approximate halving of the number of data collection decisions per OOI found. Note that the number of OOIs in the field in that run was also smaller than the usual count of seven or eight.

% The UGVs don't have stringent compute constraints and hence in run 6 we utilised the full NATS algorithm in a team of two UGVs. 

% However, the two UGVs found three and five OOIs respectively in the face of incorrect information. 
% The number of unique OOIs from these eight detections was six. 

% The false positive rate was high in this run, however the algorithm was robust to that as well. The last remaining OOI which was not found was on top of a hill and therefore invisible to UGVs.

% In presence of the detector failure the coverage algorithm on robots with a working detector would have skipped cells with OOIs in them considering them visited. 
